# Supplementary material for: SC-ML: Self-supervised Counterfactual Metric Learning for Debiased Visual Question Answering
Source: arXiv:2304.01647 source file (2023-04-04)
Supplement: Supplementary file 1 [file appendix.pdf]

## Appendix

Visualizations for the baseline (LXMERT) and SS-DML method (as shown in Fig.7), and the blue area shows the

language bias (language prior) present in the current question. SS-DML decreases the difficulty of understanding the image by masking the interfering visual features, and effectively mitigates the language bias.

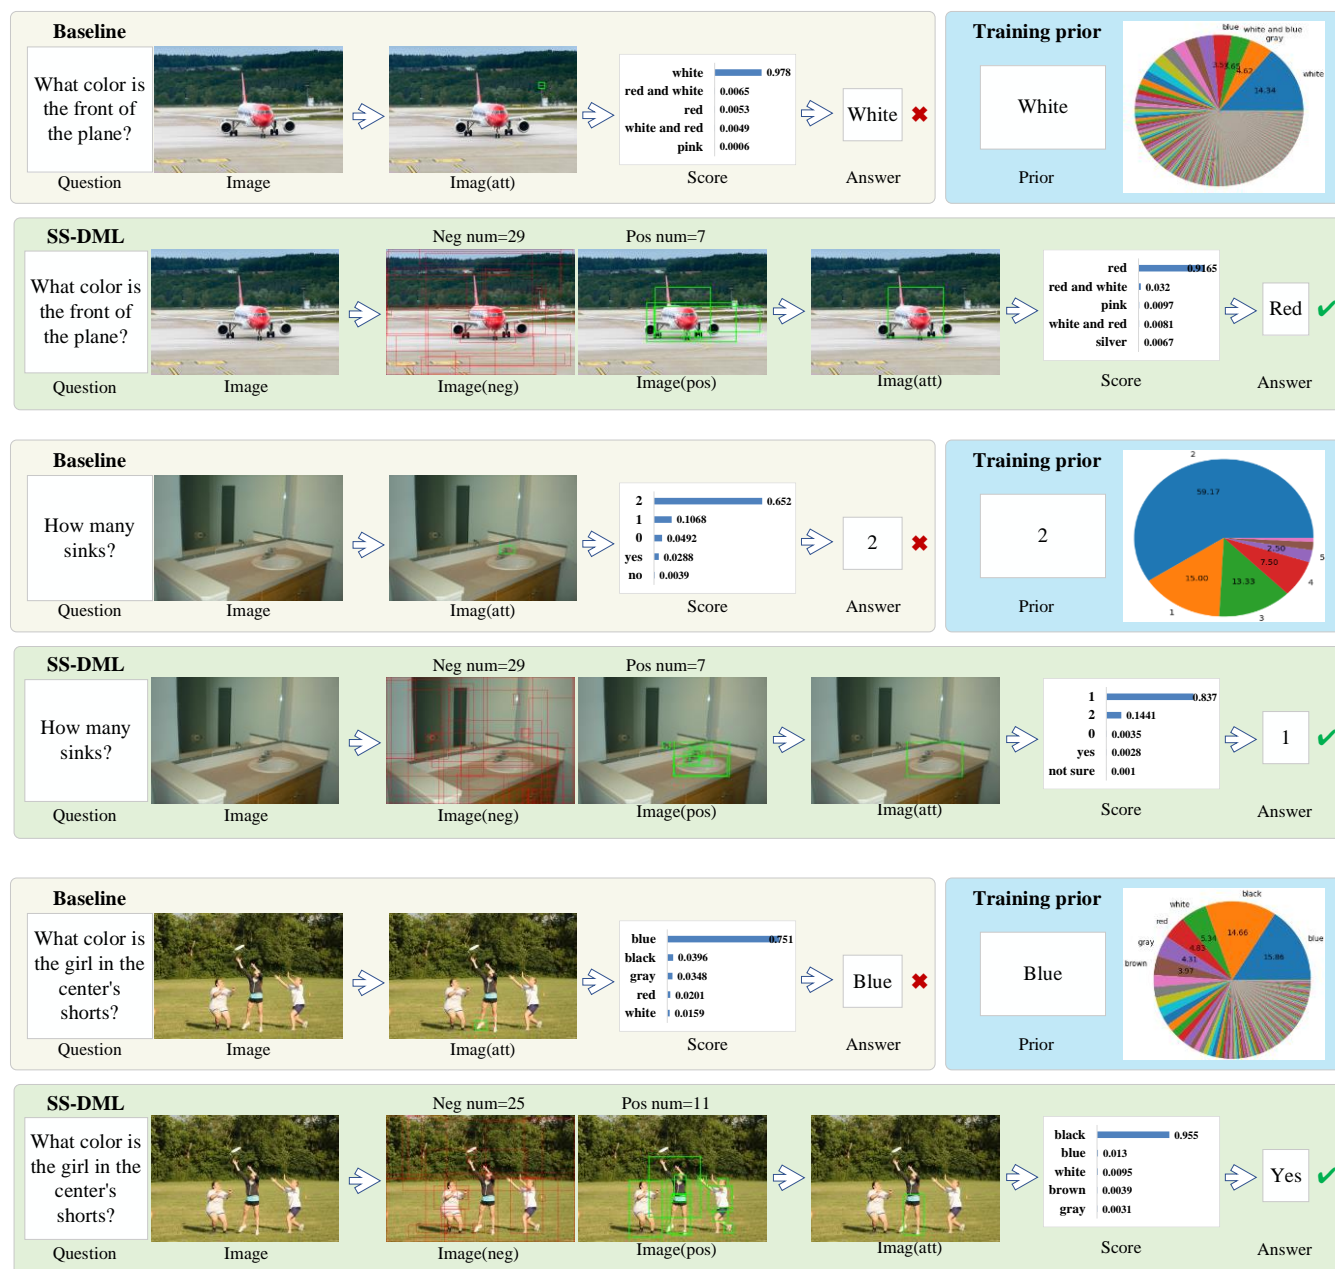

**Baseline**

Question: How many sinks?

Image:

Image(att):

Score:

|     |        |
|-----|--------|
| 2   | 0.652  |
| 1   | 0.1068 |
| 0   | 0.0492 |
| yes | 0.0288 |
| no  | 0.0039 |

Answer: 2 ❌

**Training prior**

Prior: 2

**SS-DML**

Question: How many sinks?

Image:

Image(neg):

Image(pos):

Image(att):

Score:

|          |        |
|----------|--------|
| 1        | 0.837  |
| 2        | 0.1441 |
| 0        | 0.0035 |
| yes      | 0.0028 |
| not sure | 0.001  |

Answer: 1 ✔️

**Baseline**

Question: What color is the girl in the center's shorts?

Image:

Image(att):

Score:

|       |        |
|-------|--------|
| blue  | 0.751  |
| black | 0.0396 |
| gray  | 0.0348 |
| red   | 0.0201 |
| white | 0.0159 |

Answer: Blue ❌

**Training prior**

Prior: Blue

**SS-DML**

Question: What color is the girl in the center's shorts?

Image:

Image(neg):

Image(pos):

Image(att):

Score:

|       |        |
|-------|--------|
| black | 0.955  |
| blue  | 0.013  |
| white | 0.0095 |
| brown | 0.0039 |
| gray  | 0.0031 |

Answer: Yes ✔️

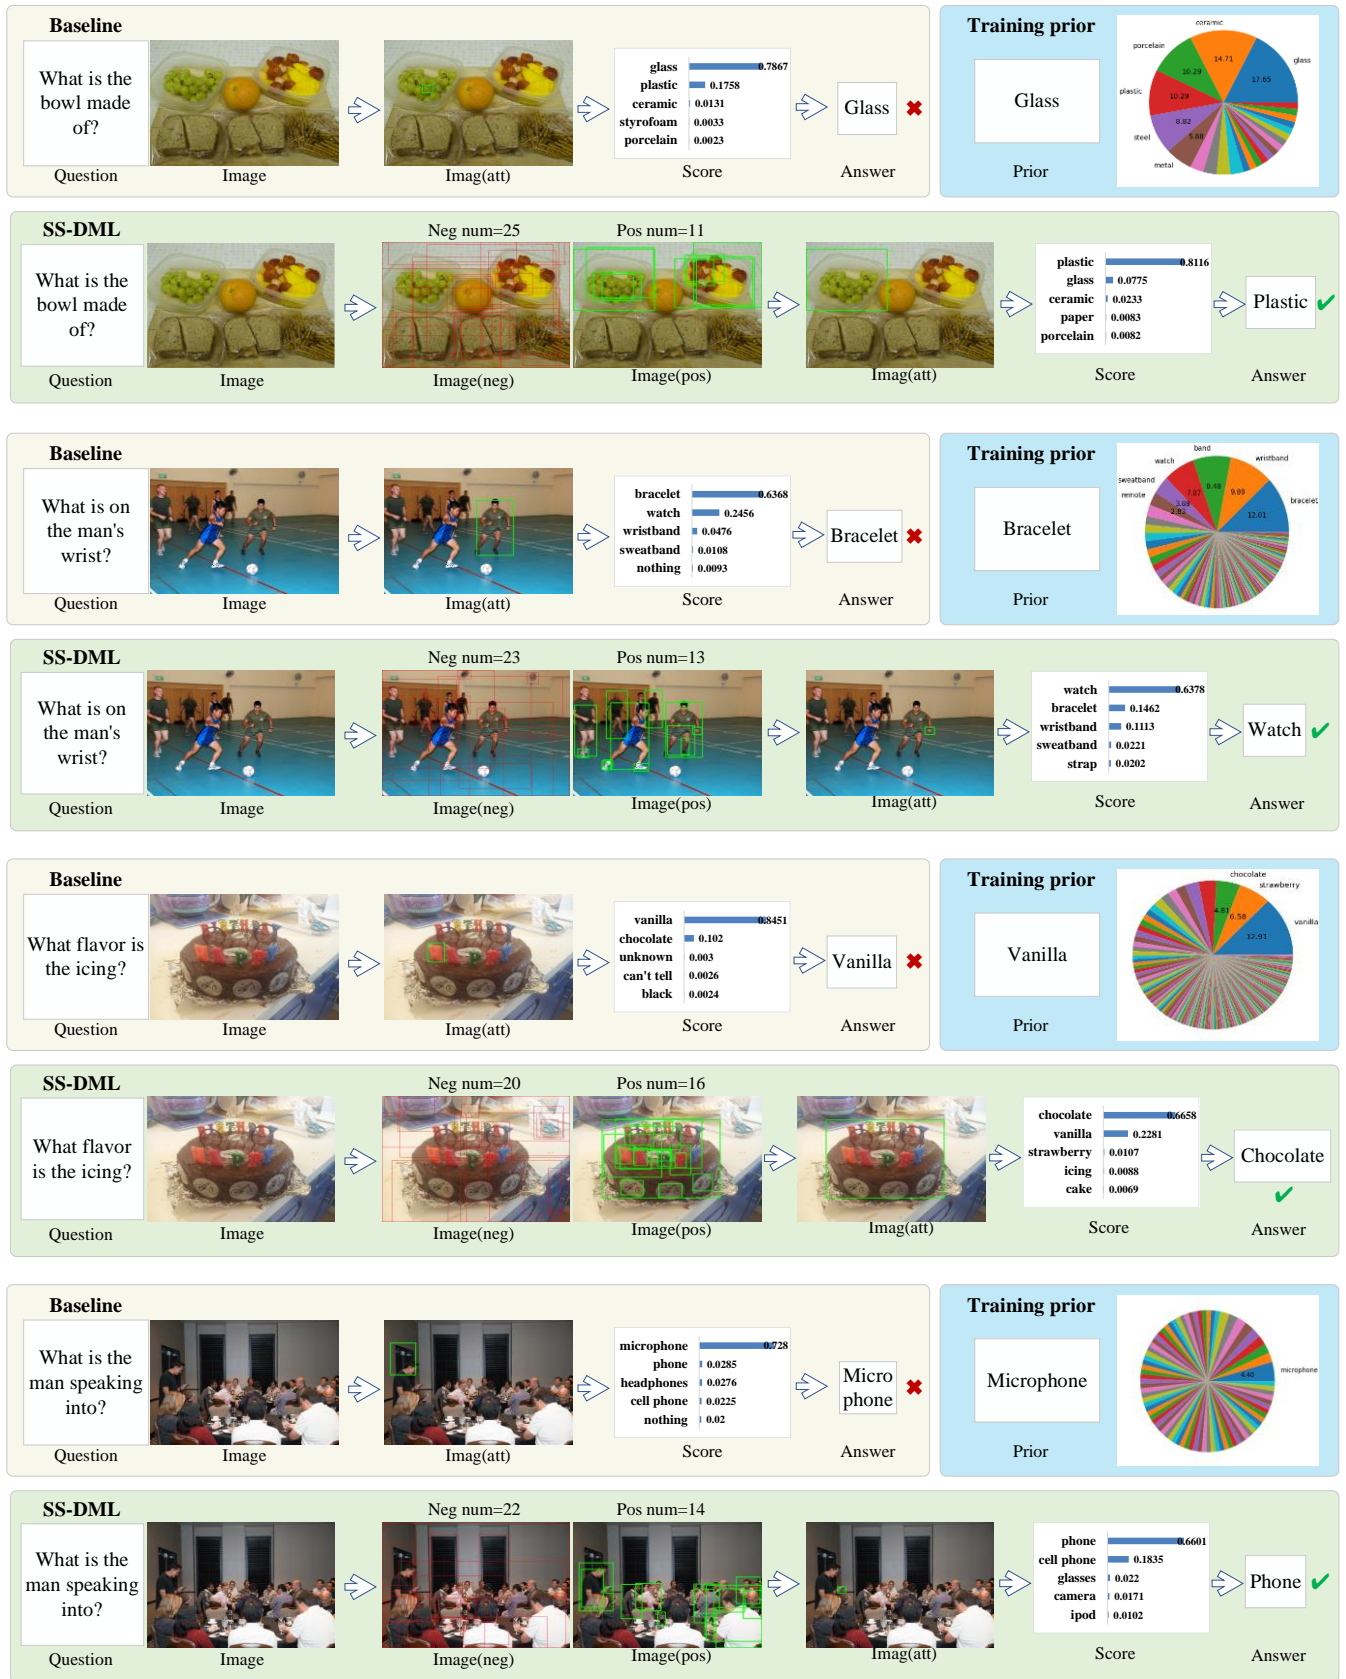

**Baseline**

What is on the man's wrist?

Image

Image(att)

|           |        |
|-----------|--------|
| bracelet  | 0.6368 |
| watch     | 0.2456 |
| wristband | 0.0476 |
| sweatband | 0.0108 |
| nothing   | 0.0093 |

Score

Answer: Bracelet ❌

**Training prior**

Prior: Bracelet

**SS-DML**

What is on the man's wrist?

Image

Image(neg) Neg num=23

Image(pos) Pos num=13

Image(att)

|           |        |
|-----------|--------|
| watch     | 0.6378 |
| bracelet  | 0.1462 |
| wristband | 0.1113 |
| sweatband | 0.0221 |
| strap     | 0.0202 |

Score

Answer: Watch ✅

**Baseline**

What flavor is the icing?

Image

Image(att)

|            |        |
|------------|--------|
| vanilla    | 0.8451 |
| chocolate  | 0.102  |
| unknown    | 0.003  |
| can't tell | 0.0026 |
| black      | 0.0024 |

Score

Answer: Vanilla ❌

**Training prior**

Prior: Vanilla

**SS-DML**

What flavor is the icing?

Image

Image(neg) Neg num=20

Image(pos) Pos num=16

Image(att)

|            |        |
|------------|--------|
| chocolate  | 0.6658 |
| vanilla    | 0.2281 |
| strawberry | 0.0107 |
| icing      | 0.0088 |
| cake       | 0.0069 |

Score

Answer: Chocolate ✅

**Baseline**

What is the man speaking into?

Image

Image(att)

|            |        |
|------------|--------|
| microphone | 0.728  |
| phone      | 0.0285 |
| headphones | 0.0276 |
| cell phone | 0.0225 |
| nothing    | 0.02   |

Score

Answer: Microphone ❌

**Training prior**

Prior: Microphone

**SS-DML**

What is the man speaking into?

Image

Image(neg) Neg num=22

Image(pos) Pos num=14

Image(att)

|            |        |
|------------|--------|
| phone      | 0.6601 |
| cell phone | 0.1835 |
| glasses    | 0.022  |
| camera     | 0.0171 |
| ipod       | 0.0102 |

Score

Answer: Phone ✅

Figure 7: Visualizations for mitigating the language bias.
